# Supplementary material for: Prescriptive Cluster-Dependent Support Vector Machines with an Application to Reducing Hospital Readmissions
Source: arXiv:1903.09056 source file (2019-03-21)
Supplement: Supplementary file 1 [file appendix_prescriptiveSVM.tex]

\begin{equation*}  
\begin{array}{r@{}l}
\min_{\hat{\mathbf x
}_i, \xi_i^l} \quad  & 
\frac{1}{N^+} \sum\limits_{i=1}^{N^+} (\lambda \xi_i^l+ \| \hat{\mathbf x
}_{i} -\mathbf x
_{i}\|^p_p ) \\
s.t. \quad  &
\beta_0^l+ (\boldsymbol{\beta}_d^l)^{'} \hat{\mathbf x
}_{i} \leq \xi_i^l-1, %\sum\limits_{k \neq l} z_{ik} , -M(1-z_{il})
 \forall i \in {N^+},\\ %\forall l,
&
\hat{x}_{i,d}=x_{i,d}, \forall d \in U,  \\
%\quad uncontrollable \\
&
\xi_i^l \geq 0,\\
&
L_{i,d} \leq \hat{x}_{i,d} \leq U_{i,d}, \forall d \in C. %, \quad controllable 
%     -(x_new'*wtrain+btrain)-1 +e >=0;   %:alphatrain;
%     e>=0; %slack
%     x_new(control_id)>=hct_lb;
%     x_new(control_id)<=hct_ub;
%     x_new(control_id_mask>0)==x(control_id_mask>0);
\end{array}
\end{equation*}
which can be decoupled into $N^+$ subproblems, $\forall i \in {N^+}$,

\begin{equation*}  
\begin{array}{r@{}l}
\min_{\hat{\mathbf x
}_i, \xi_i^l} \quad  & 
\lambda \xi_i^l+ \| \hat{\mathbf x
}_{i} -\mathbf x
_{i}\|^p_p  \\
s.t. \quad  &
\beta_0^l+ (\boldsymbol{\beta}_d^l)^{'} \hat{\mathbf x
}_{i} \leq \xi_i^l-1, %\sum\limits_{k \neq l} z_{ik} , -M(1-z_{il})
\\ %\forall l, \forall i,
&
\hat{x}_{i,d}=x_{i,d}, \forall d \in U, \\
&
\xi_i^l \geq 0,\\
&
L_{i,d} \leq \hat{x}_{i,d} \leq U_{i,d}, \forall d \in C
\end{array}
\end{equation*}
